# Supplementary material for: Evidence of a critical hole concentration in underdoped YBa$_2$Cu$_3$O$_y$ single crystals revealed by $^{63}$Cu NMR
Source: arXiv:1212.0530 source file (2012-12-03)
Supplement: Supplementary file 1 [file YBCO_NMR_supple.pdf]

| compound | $T_c$ (K) | $c$-axis (Å) | hole doping $p$ |
|---|---|---|---|
| $YBCO_{6.35}$ | 10 | 11.781(1) | 0.062(2) |
| $YBCO_{6.4}$ | 21 | 11.768(1) | 0.075(2) |
| $YBCO_{6.45}$ | 35 | 11.761(1) | 0.082(2) |
| $YBCO_{6.5}$ (short) | 53 | 11.738(1) | 0.106(2) |
| $YBCO_{6.5}$ (long) | 61 | 11.731(1) | 0.114(2) |
| $YBCO_{6.6}$ | 61 | 11.715(1) | 0.135(2) |

TABLE I: Superconducting transition temperature, $T_c$, lattice parameter, $c$, and hole doping, $p$, for the different doping levels.

## SAMPLE PREPARATION AND CHARACTERIZATION

The samples used in this study are the same as in ref. [1], and references therein. The oxygen content, the superconducting transition temperature, $T_c$, the $c$-axis lattice constant, and the hole concentration, $p$, are given in Table I. The hole concentration was determined from the $c$-axis parameter according to ref. [2].

The typical sample mass and size was $\sim$ 10 mg and $a \times b \times c = 2.7 \times 2 \times 0.5$ mm. The oxygen content was controlled by annealing the samples at a fixed oxygen partial pressure [3]. The detwinning was achieved by application of uniaxial mechanical stress along the crystallographic (1,0,0) direction [1]. The sample $YBCO_{6.5}$ (short) has a relatively short ortho-II correlation length, whereas $YBCO_{6.5}$ (long) was improved for a longer correlation length of $\sim$ 100 Åperpendicular to the chains, i.e. along the $a$-axis. The lower doping levels are of course not well ordered, and should exhibit oxygen vacancies in the chains due to the lower oxygen concentration.

## ADDITIONAL NMR SPECTRA

In the following, additional NMR spectra are shown including the full temperature dependence of the samples $YBCO_{6.5}$ (short) and $YBCO_{6.6}$ (Fig. S1), and $YBCO_{6.4}$ (Fig. S3), and a comparison of the spectra at 290 K for all different doping levels (Fig. S2).

Fig. S4 shows the spectra measured with different repetition times of the pulse sequence

for $YBCO_{6.4}$ at $T = 120$ K $< T_0$ and at $T = 290$ K $> T_0$. Below $T_0$, the figure indicates that those parts of the spectrum are suppressed by a short repetition time, which arise from sp0. In contrast, the planar Cu(2) signal [the intensity below 80.5 MHz comes only from Cu(2)] as well as the full chain site $Cu(1)_2$ are only slightly affected by the fast repetition time. Therefore, this figure indicates that the long relaxation rate $(T_{1\ell}T)^{-1}$ arises from the new spectrum sp0, whereas the short relaxation rate $(T_{1s}T)^{-1}$ arises from the planar Cu(2) line.

Fig. S5 shows field dependent spectra of $YBCO_{6.4}$ at 120 K. The field dependence indicates that the EFG at the sp0 sites is not directed along the $c$-axis, and probably has a large anisotropy parameter, $\eta$. We confirmed this symmetry of the EFG for sp0 also by measurements for $H \parallel b$ (not shown). Although this is a similar symmetry as for $Cu(1)_2$, we think that sp0 does not originate from the chains for the following reasons:

(i) sp0 can not be a full chain site $Cu(1)_2$ nor a satellite of $Cu(1)_2$. First of all, sp0 emerges in the spectra with decreasing temperature, whereas $Cu(1)_2$ is always clearly visible. Secondly, $Cu(1)_2$ has a short spin lattice relaxation time $T_1$. This is also visible in Fig. S4 where sp0 emerges with increasing repetition time of the pulse sequence, whereas the intensity of $Cu(1)_2$ hardly changes with different repetition times. The satellites of $Cu(1)_2$ can fall into the frequency region of Cu(2) and sp0 for $H \parallel c$, too, since $\eta$ is close to one for this site and the main component of the EFG points along the $a$-axis. For $H \parallel b$ the satellites are far away, but still we observe sp0 in the spectra (not shown). Also, the satellites of the full chains are expected to be quite broad due to the oxygen disorder [4, 5]. Only for $YBCO_{6.5}$ with a long chain correlation length, the satellites may be visible and narrow, but sp0 appears only below this doping level.

(ii) The Cu chain site with only one oxygen, $Cu(1)_1$, i.e., the end Cu ion of the oxygen-filled chain, could be responsible for sp0. This site has never been observed in the Cu NMR spectra of YBCO [6]. If $Cu(1)_1$ is responsible for sp0, one should expect an average chain length involving only $\sim 4$ Cu atoms, since the amplitude of sp0 and $Cu(1)_2$ are comparable to each other (see Fig. 1, or S3 and S5). We consider that this is unlikely, also because a three oxygen-coordinated Cu, i.e. $Cu(1)_1$, is chemically unfavorable.

Finally, we would like to point out that the planar Cu site should consist of two sites as well, one planar copper that is below an empty chain and one that is below a full chain. The central NMR signal of these sites for $H \parallel c$ can be distinguished only for samples with

$y \sim 6.5$ and long chain correlation lengths and at very low temperatures, or for $H \parallel a$ or $b$ [5, 6]. On the other hand, the satellites can be well separated, since they have different quadrupole frequencies. In principle, different quadrupole frequencies do not lead to different central transitions for $H \parallel c$, the direction parallel to the main component of the EFG. One possible explanation would be that the EFG of the planar signal below the empty chains is tilted. This has been suggested by Ofer et al. [7], who found a tilt of $\sim 20°$. However, a simulation of the central transition at $H = 7$ T assuming a tilt of $20°$ of the EFG would lead to a splitting of more than 1.5 MHz for both planar sites, which is two orders of magnitude more than experimentally observed [5]. Nevertheless, it is not clear if sp0 can be related to either the planar site below an empty or a filled chain. A tilt of the EFG at sp0 and/or a change of $\eta$ would at least explain the peculiar field dependence in Fig. S5.


[1] D. Haug, V. Hinkov, Y. Sidis, P. Bourges, N. B. Christensen, A. Ivanov, T. Keller, C. T. Lin, and B. Keimer, New J. Phys. **12**, 105006 (2010).

[2] R. Liang, D. A. Bonn, and W. N. Hardy, Phys. Rev. B **73**, 180505 (2006).

[3] J. D. Jorgensen, B. W. Veal, A. P. Paulikas, L. J. Nowicki, G. W. Crabtree, H. Claus, and W. K. Kwok, Phys. Rev. B **41**, 1863 (1990).

[4] A. Erb, A. Manuel, M. Dhalle, F. Marti, J.-Y. Genoud, B. Revaz, A. Junod, D. Vasumathi, S. Ishibashi, A. Shukla, et al., Solid State Commun. **112**, 245 (1999).

[5] T. Wu, H. Mayaffre, S. Kramer, M. Horvatic, C. Berthier, W. N. Hardy, R. Liang, D. A. Bonn, and M.-H. Julien, Nature **477**, 191 (2011).

[6] Z. Yamani, W. A. MacFarlane, B. W. Statt, D. Bonn, R. Liang, and W. N. Hardy, Physica C **405**, 227 (2004).

[7] R. Ofer and A. Keren, Phys. Rev. B **80**, 224521 (2009).

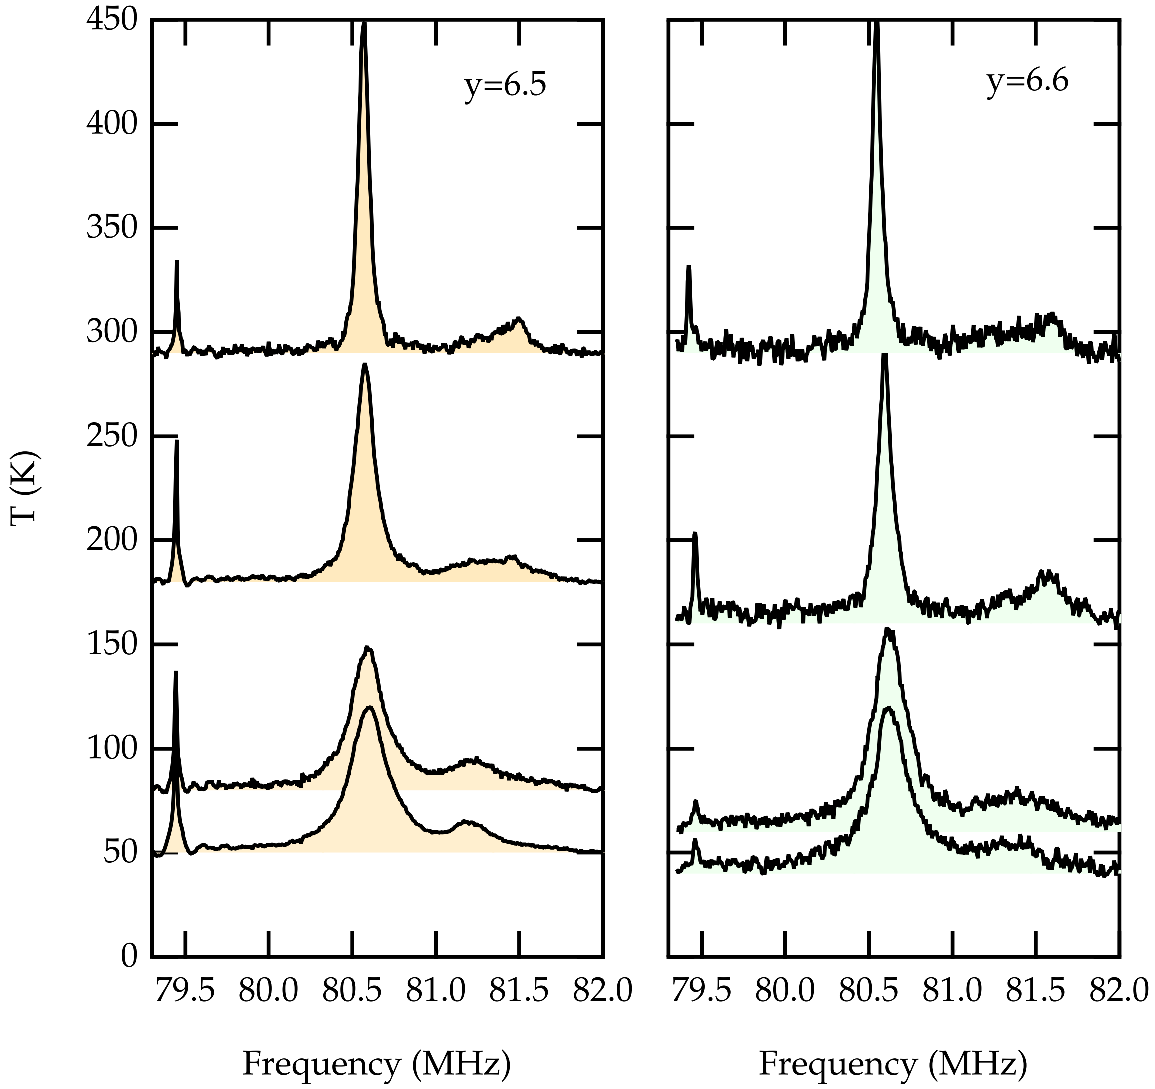


FIG. 1: $^{63}$Cu NMR spectra in YBCO$_y$ at the external field of 7.049 T along the $c$-axis for $y$=6.5 (short) (left panel) and 6.6 (right panel). The repetition time during the measurements was on the order of the longest $T_1$ we observed at each temperature. The Cu(1)$_0$ site (left peak), which also has a long $T_1$, appears smaller in the spectra since it is at the edge of the spectra, where it was only partly excited by the pulses. The Cu(2) signal is a composite of planar Cu sites, which are below empty and filled chains. These sites can be distinguished only for samples with $y \sim 6.5$ and long chain correlation lengths and at very low temperatures, or for $H \parallel a$ or $b$ [5, 6].

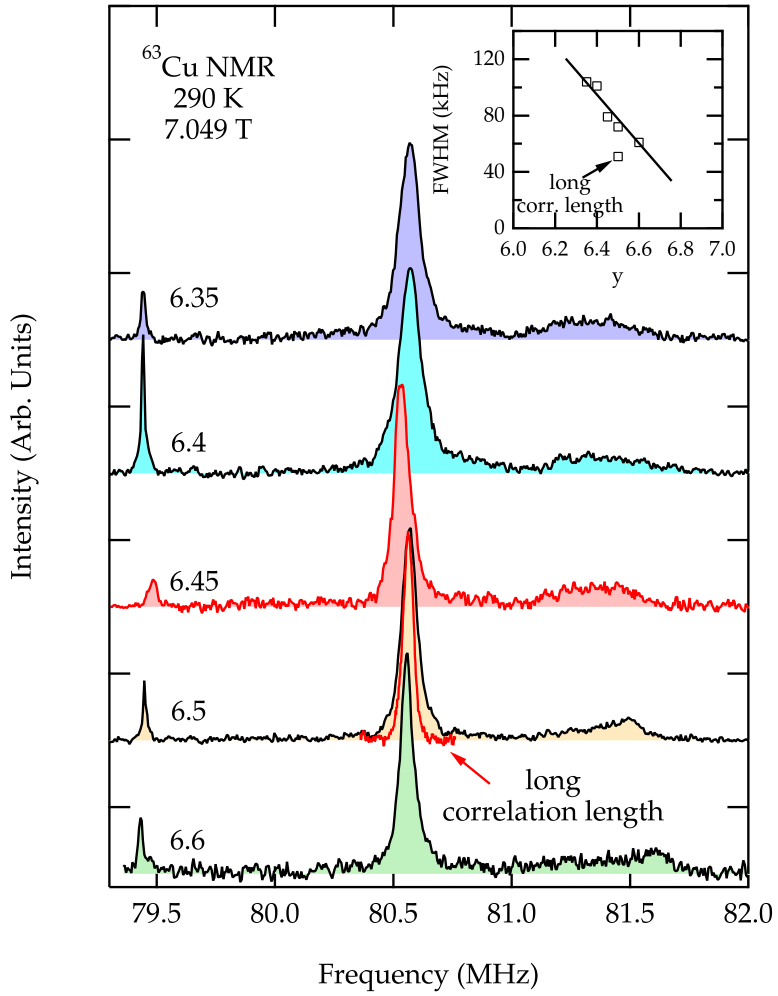


FIG. 2: Comparison of the $^{63}$Cu spectra at 290 K in YBCO$_y$ as a function of oxygen content $y$. Note, that the Cu(2) spectra for $y$=6.45 is slightly shifted due to a small misalignment of the sample with respect to the $c$-axis. This angular dependent shift comes mainly from the second order quadrupole effect, which is zero for exactly $H \parallel c$. The inset shows the full width at half maximum (FWHM) of the planar Cu(2) spectrum versus $y$. The $y$-dependence of the FWHM indicates that the line broadening mechanism is dominated by the inherent oxygen disorder in the chains, rather than impurities. This is supported by the narrow line width of the $y$=6.5 sample with a long chain correlation length.

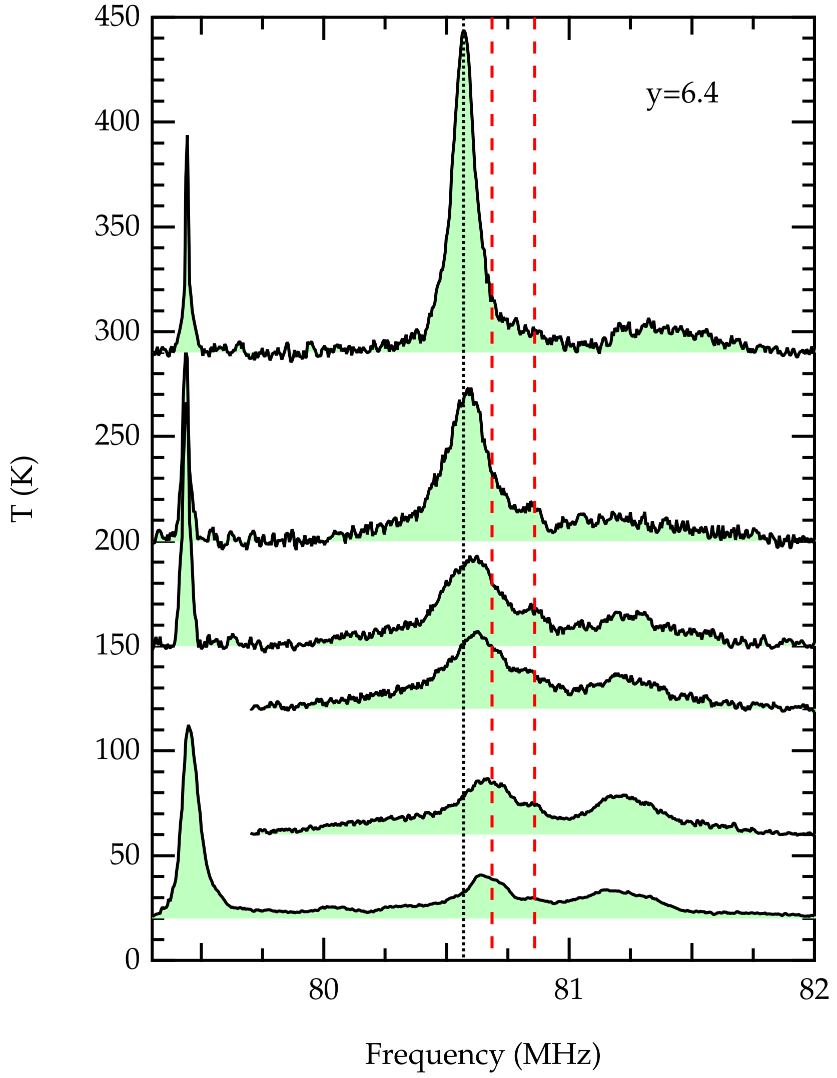


FIG. 3: $^{63}$Cu NMR spectra in YBCO$_{6.4}$ as a function of temperature at the external field of 7.049 T applied along the $c$-axis.

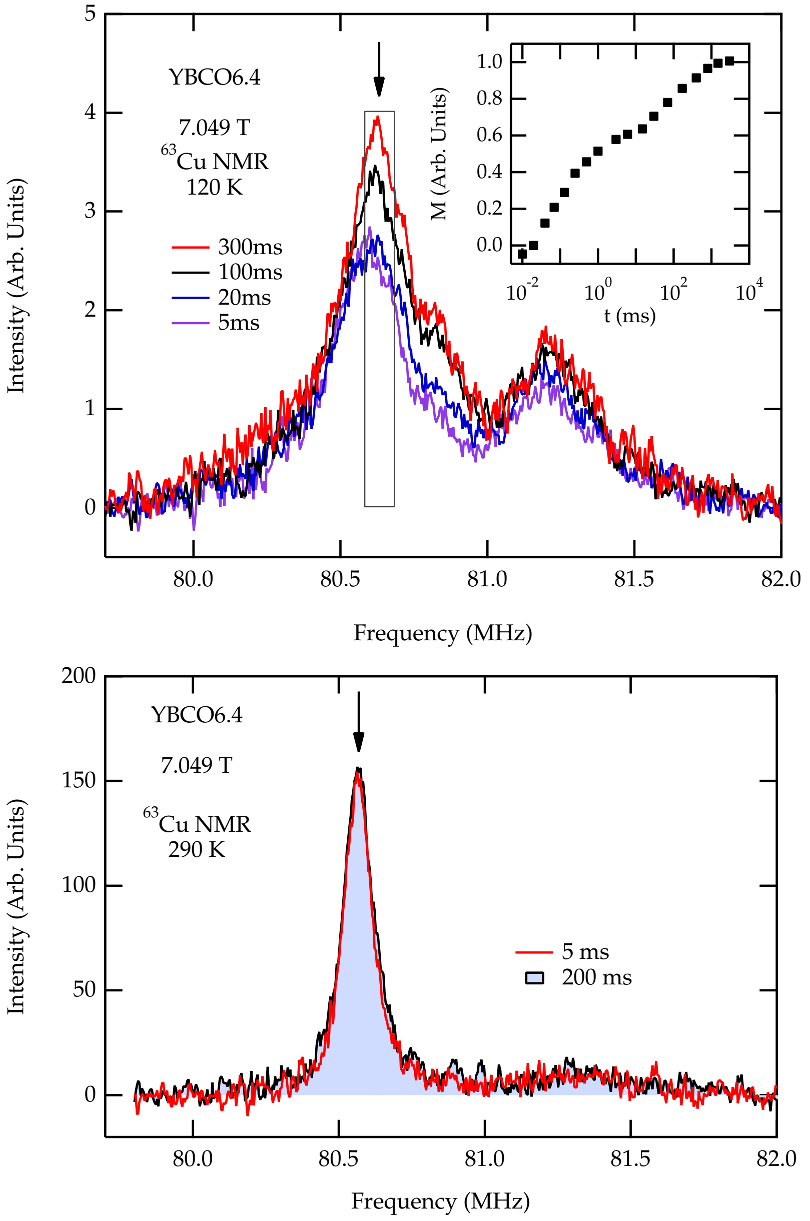


FIG. 4: $^{63}$Cu NMR spectra in YBCO$_{6.4}$ at 7.049 T along the $c$ axis at 120 K $< T_0$ (upper panel) and at 290 K $> T_0$ (lower panel) with different repetition times. Down arrows denote the resonance frequency at which the relaxation rates were measured. Inset: the nuclear magnetization data obtained by integrating the partial spectral area around the resonance frequency, as represented by rectangle. This figure suggests that the long relaxation rate $(T_{1\ell}T)^{-1}$ arises from the new spectrum sp0.

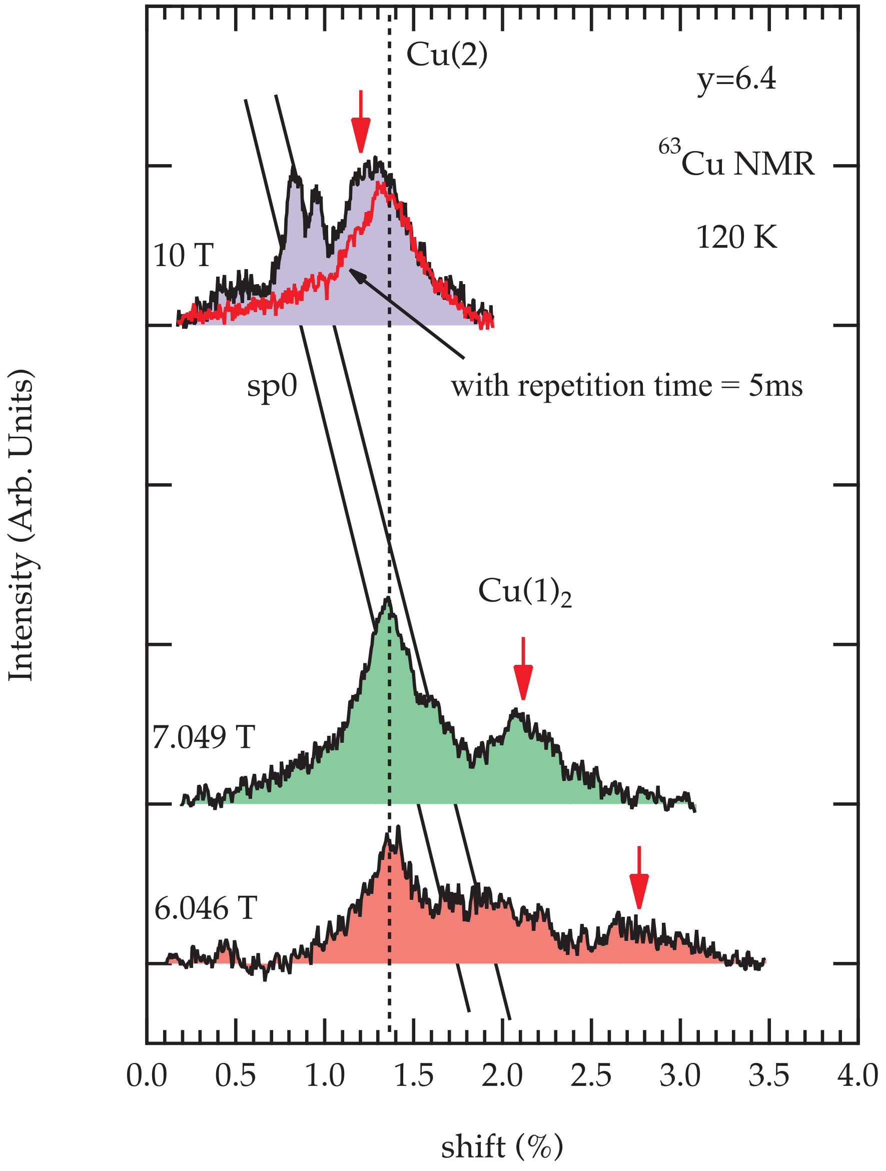


FIG. 5: $^{63}$Cu NMR spectra in YBCO$_{6.4}$ at 120 K at three different external fields along the $c$ axis in terms of the NMR shift. As expected, Cu(2) does not shift, but Cu(1)$_2$ and the sp0 line reveal a strong field dependence. Down arrows denote the resonance frequencies of Cu(1)$_2$ obtained from simulations based on parameters for Cu(1)$_2$ taken from [6]. Solid lines are guides to the eye for sp0. Two peaks are clearly visible at 10 T, which are completely suppressed by a fast repetition time (red line), providing one more evidence that sp0 represents a new phase characterized by a very long $T_1$. In addition, this field dependence indicates that the EFG at the sp0 sites is not directed along the $c$-axis.
